# Supplementary material for: Kinetic mechanism for reversible structural transition in MoTe2 induced by excess charge carriers
Source: arXiv:1711.11147 source file (2018-04-25)
Supplement: Supplementary file 1 [file supplementary-info.pdf]

# Kinetic mechanism for reversible structural transition in $MoTe_2$ induced by excess charge carriers (supplementary information)

O. Rubel*
*Department of Materials Science and Engineering, McMaster University,*
*1280 Main Street West, Hamilton, Ontario L8S 4L8, Canada*
(Dated: November 28, 2017)

TABLE S1. Structural parameters of 2H, 1T and 1T' phases of bulk $MoTe_2$ obtained using DFT. The experimental data[1,2] are given in square brackets for comparison.

| Phase | Space group | Lattice parameters (Å) | | | Angles (deg.) | | | Fractional coordinates |
|---|---|---|---|---|---|---|---|---|
| | | $a$ | $b$ | $c$ | $\alpha$ | $\beta$ | $\gamma$ | |
| 2H | $P6_3/mmc$, no. 194 | 3.513 | 3.513 | 14.473 | 90 | 90 | 120 | $u_{\text{Mo}} = (1/3, 2/3, 0.2496)$ |
| | | [3.519] | [3.519] | [13.964] | | | | $u_{\text{Te}} = (1/3, 2/3, 0.6256)$ |
| 1T | $P\bar{3}m1$, no. 162 | 3.46 | 3.46 | 15.13 | 90 | 90 | 120 | $u_{\text{Mo}} = (1/3, 2/3, 0.2496)$ |
| | | | | | | | | $u_{\text{Te(1)}} = (1/3, 2/3, 0.6152)$ |
| | | | | | | | | $u_{\text{Te(2)}} = (0, 0, 0.8584)$ |
| 1T' | $P2_1/m$, no. 11 | 6.391 | 3.371 | 14.73 | 90 | 93.45 | 90 | $u_{\text{Mo(1)}} = (0.1848, 1/4, 0.0056)$ |
| | | [6.33] | [3.469] | [13.86] | | [93.55] | | $u_{\text{Mo(2)}} = (0.3168, 3/4, 0.5052)$ |
| | | | | | | | | $u_{\text{Te(1)}} = (0.5805, 1/4, 0.0998)$ |
| | | | | | | | | $u_{\text{Te(2)}} = (0.0945, 3/4, 0.1390)$ |
| | | | | | | | | $u_{\text{Te(3)}} = (0.5585, 3/4, 0.3609)$ |
| | | | | | | | | $u_{\text{Te(4)}} = (0.0522, 1/4, 0.3998)$ |

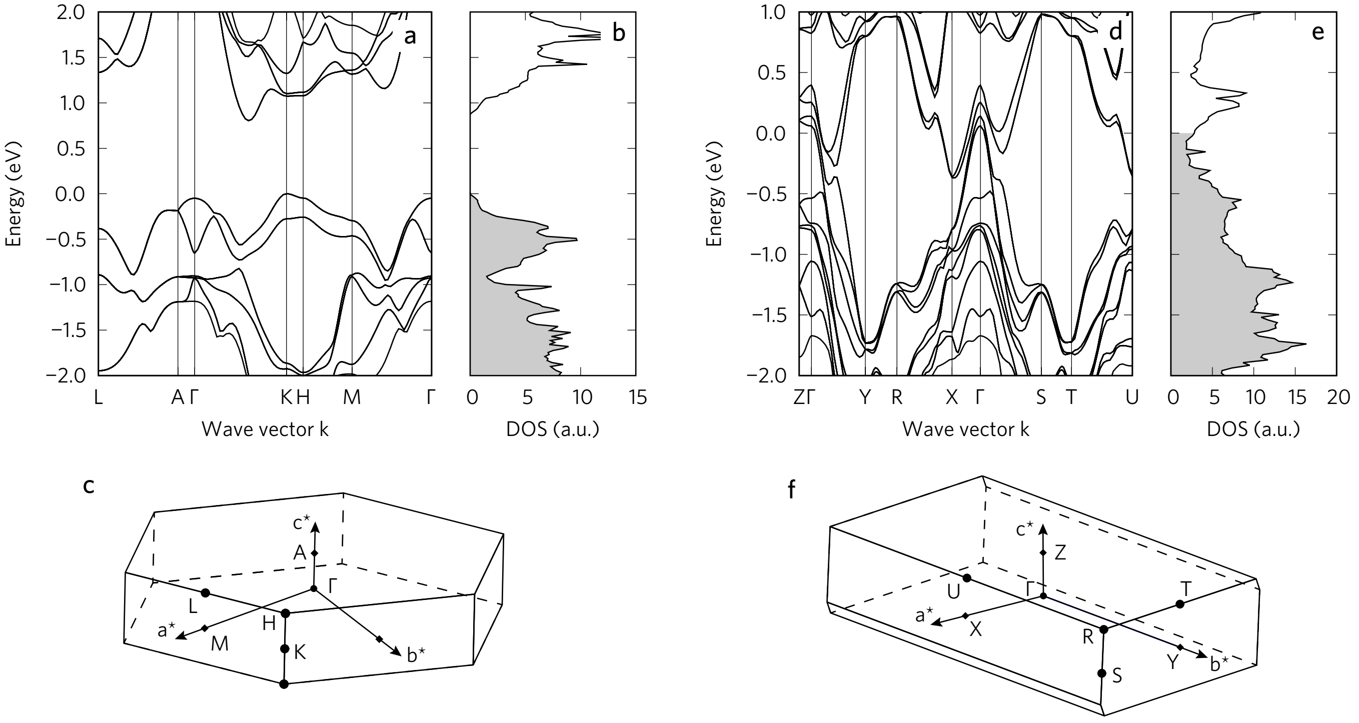


FIG. S1. Relativistic band structure and density of states (DOS) for bulk (a,b) 2H-$MoTe_2$ and (d,e) 1T'-$MoTe_2$. The origin of an energy scale is set at the Fermi energy. The corresponding Brillouin zones with high-symmetry points are shown on the panels (c) and (f).

* rubelo@mcmaster.ca

[1] D. Puotinen and R. E. Newnham, Acta Cryst. **14**, 691 (1961).
[2] B. E. Brown, Acta Cryst. **20**, 268 (1966).
